# Supplementary material for: ACE: Abstract Consensus Encapsulation for Liveness Boosting of State Machine Replication
Source: arXiv:1911.10486 source file (2019-11-24)
Supplement: Supplementary file 1 [file ACE-Supplemental_Material.pdf]

# ACE: Abstract Consensus Encapsulation for Liveness Boosting of State Machine Replication \*\*Supplemental Material\*\*

Anonymous Author(s)

## 1 Single-Shot Agreement Correctness Proof (Section 5.1)

We prove that Algorithm 1 satisfies Agreement, Termination, Validity, and Fairness properties in the asynchronous communication model. We start by proving the Agreement and Validity properties.

**Observation 1.** *The chosen LBV instances in Algorithm 1 form a properly composed execution.*

**Lemma 1.** *Algorithm 1 satisfies the Validity and Agreement.*

*Proof.* By the code, correct parties only decide on values returned from a wedge&exchange method invoked on one of the chosen instances. Therefore, by Observation 1, the Validity and Agreement properties follow from the Safety properties required by the LBV abstraction.  $\square$

We now prove that Algorithm 1 satisfies Termination. We start by showing that no honest party is stuck forever in a wave.

**Claim 1.** *Consider a wave  $k \geq 1$  that all correct parties start, then at least one barrier-sync invocation by a correct party eventually returns.*

*Proof.* Assume by way of contradiction that no barrier-sync () invocations by correct party eventually returns in wave  $k$ . Thus, no correct party ever invoke wedge&exchange in wave  $k$ . Therefore, since all correct parties invoke engage in all LBV instances in wave  $k$ , we get by the Engage-Termination property that all *propose* invocation by correct parties eventually return, and thus all correct parties eventually send ENGAGE-DONE messages to all correct leaders. Hence, all correct leaders eventually get  $n - f$  ENGAGE-DONE messages, and thus eventually invoke barrier-ready. The contradiction follows from the B-Termination property.  $\square$

**Claim 2.** *For every wave  $k \geq 1$ , if all correct parties start wave  $k$ , then all correct parties eventually complete wave  $k$ .*

*Proof.* By Claim 1, some barrier-sync invocation by a correct party eventually returns in wave  $k$ . Thus, by the B-Agreement property, all barrier-sync invocations by correct parties eventually return in wave  $k$ , and thus all correct parties eventually

invoke elect in wave  $k$ . By the L-Termination property, all elect invocations by correct parties eventually return in wave  $k$ . Therefore, the Claim follows from the Wedge&Exchange-Termination property.  $\square$

The next corollary follows by inductively applying Claim 2.

**Corollary 1.** *For every  $k \geq 1$ , all parties eventually complete wave  $k$  in Algorithm 1.*

For the rest of the proof we say that an LBV instance is *completed* if at least  $f + 1$  engage innovations by correct parties previously returned. We next bound the probability to choose a leader of a completed LBV instance.

**Claim 3.** *For every wave  $k \geq 1$ , at least  $f + 1$  LBV instances with correct leaders are completed before some correct party invokes elect.*

*Proof.* Consider some correct party that invokes elect at wave  $k$ . By the code, its barrier-sync invocation was previously returned, and thus by the B-Coordination property, at least  $f + 1$  correct parties previously invoked barrier-ready. Therefore, at least  $f + 1$  correct parties received  $n - f$  ENGAGE-DONE messages, at least  $f + 1$  of which are from correct parties. Since correct parties send ENGAGE-DONE messages to party  $p_j$  only after their engage invocation in the LBV instance in which  $p_j$  acts as leader returns, at least  $f + 1$  LBV instances with correct leaders are completed before some correct party invokes elect.  $\square$

**Claim 4.** *Consider a wave  $k \geq 1$  that all parties start, the probability for all correct parties to decide at wave  $k$  is at least  $\frac{f+1}{n}$ .*

*Proof.* By Corollary 1, all correct parties invoke elect in view  $k$  and, by the L-Agreement property, all invocations return the same leader. By Claim 3, at least  $f + 1$  LBV instances are completed before some correct party invokes elect at view  $k$ . Therefore, by the L-Validity and L-Unpredictability properties, we get that the probability to choose a leader of a completed LBV instance is at least  $\frac{f+1}{n}$ . By the Completeness property of the LBV abstraction, if a completed LBV instance is chosen, then no wedge&exchange invocation by correct party returns  $v = \perp$ . Therefore, by the code, all correct parties decide at the end of wave  $k$  with probability  $\frac{f+1}{n}$ .  $\square$

**Lemma 2.** *Algorithm 1 satisfies Termination.*

*Proof.* By Corollary 1, correct parties are never stuck indefinitely in any view, and thus all honest parties eventually start all views. Therefore, by Claim 4, all honest parties eventually decide with probability 1. Moreover, the expected number of views after which all correct party decide is  $\frac{n}{f+1}$ .  $\square$

**Lemma 3.** *Algorithm 1 satisfies Fairness.*

*Proof.* By the Completeness property of the LBV abstraction, if a completed instance is chosen, then all correct parties decide at the end of the wave. By Claim 3, for every wave  $k \geq 1$ , at least  $f + 1$  LBV instances with correct leaders are completed before a unique instance is chosen in the wave. Therefore, even if all LBV instances with faulty parties have been completed as well, the probability to decide on value proposed by a correct party is at least  $1/2$ . Moreover, during synchronous periods, all instances with correct parties complete with equal probability, and thus by the L-validity, all correct parties have an equal probability for their values to be chosen.  $\square$

## 2 Partially Synchronous Algorithm Reconstruction (Section 5)

For completeness, we show how to use the LBV abstraction to reconstruct a variant of the partially synchronous base Agreement algorithm that the LBV abstraction was instantiated with. To this end, we assume the base algorithm provides two methods: *getLeader* and *getTimeout*. These methods should implement the logic used by the base algorithm to map designated leaders to views and set their timeouts, respectively. In particular, *getLeader*( $v$ ) gets a view  $v$  and returns a party  $p_i \in \{p_1 \dots p_n\}$ , and *getTimeout*( $v, S$ ) gets a view  $v$  together with a state  $S$  and returns a timeout.

The pseudocode appears in Algorithm 1. The protocol proceeds in views. Timeouts are used in order to demote a leader who was unable to drive progress. At the beginning of every view, parties first get the leader and the timeout of the current view, and then invoke *engage* in the leaders LBV instance and a timer to monitor the leaders progress. If the *engage* invocation returns  $v$  before the timer expires, then  $v$  is decided. In any case, whether the *engage* invocation returns or the timer expires, a *wedge&exchange* is invoked in order to update the state and safely proceed to the next view.

Note that the algorithm forms a properly composed execution of the LBV instances, and thus Validity and Agreement are trivially satisfied by the Safety properties required by the LBV abstraction. As any protocol in the partially synchronous model, the termination of the algorithm requires a long enough synchronous period in which all correct parties execute the same view.

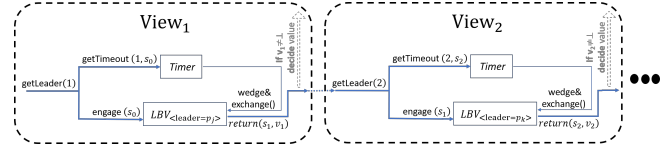

**Figure 1.** An illustration of the reconstruction of the partially synchronous algorithm. The LBV and timer are invoked in parallel at the same time; when either the LBV engage returns or the timer expires, then the parties move on to the next view, possibly deciding.

**Algorithm 1** Reconstruction of base partially synchronous single-shot agreement: protocol for party  $p_i$ .

```

1: upon ES-propose( $id, S$ ) do
2:    $state \leftarrow S$ ;  $view \leftarrow 1$ 
3:   while true do
4:      $leader \leftarrow \text{GETLEADER}(view)$ 
5:      $timeout \leftarrow \text{GETTIMEOUT}(view, state)$ 
6:     invoke engage  $\langle view, leader \rangle(state)$ 
7:     invoke a timer to expire in  $timeout$ 
8:     wait for timer to expire or engage to return
9:     if engage returned  $v$  then
10:      decide  $v$ 
11:       $\langle state, * \rangle \leftarrow \text{wedge\&exchange} \langle view, leader \rangle()$ 
12:       $view \leftarrow view + 1$ 

```

## 3 Leader-Election Implementation (Section 6.1)

The leader election is similar to that of [1] and [4]. When a party invokes *elect*, it signs the instance's identification and broadcasts its share. When a correct party collects  $f + 1$  valid shares, it combines them to a threshold signature, hashes the signature to get a pseudo random value, and returns the value modulo  $n$  to get a random leader.

As the threshold signature is generated from  $f + 1$  valid shares, all correct parties eventually generate it provided that at least  $f + 1$  correct parties invoke *elect*, satisfying *L-Termination*. Due to the nature of threshold cryptography, the generated threshold signature is the same for all correct parties [2], and since the hash and modulo functions are deterministic, all parties agree on the electing leader, satisfying *L-Agreement*. For formal analysis of *L-Validity* and *L-Unpredictability* please refer to [1, 3, 4].

## References

- [1] Ittai Abraham, Dahlia Malkhi, and Alexander Spiegelman. 2019. Asymptotically Optimal Validated Asynchronous Byzantine Agreement. In *Proceedings of the 2019 ACM Symposium on Principles of Distributed Computing (PODC '19)*. ACM, New York, NY, USA, 337–346. <https://doi.org/10.1145/3293611.3331612>

- [2] Dan Boneh, Ben Lynn, and Hovav Shacham. 2001. Short signatures from the Weil pairing. In *International Conference on the Theory and Application of Cryptology and Information Security*. Springer, 514–532.
- [3] Christian Cachin, Klaus Kursawe, Frank Petzold, and Victor Shoup. 2001. Secure and efficient asynchronous broadcast protocols. In *Annual International Cryptology Conference*. Springer, 524–541.
- [4] Christian Cachin, Klaus Kursawe, and Victor Shoup. 2000. Random Oracles in Constantinople: Practical Asynchronous Byzantine Agreement Using Cryptography. *Journal of Cryptology* 18 (2000).
